# Supplementary material for: Auditing evaluation artifacts and data leakage in large language model systems for rare disease diagnosis
Source: arXiv:2610.33592 source file (2026-10-24)
Supplement: Supplementary file 2 [file urlTable.tex]

\footnotesize % 让整张表格的字体变小。如果觉得太小，可以将其修改为 \small
\begin{tabularx}{\linewidth}{
    >{\hsize=0.2\hsize\raggedright\arraybackslash}X 
    >{\hsize=0.8\hsize\centering\arraybackslash}X 
}
    \toprule
    \textbf{Dataset} & \textbf{Access URL} \\
    \midrule
    RareArena           & https://github.com/chen/rarearena \\
    Phenopacket           & https://github.com/monarch-initiative/phenopacket-store \\
    LIRICAL    & https://zenodo.org/record/3905420 \\
    RDmaster            & https://github.com/1678492347/rdmaster-test \\
    PhenoDP                & https://link.springer.com/article/10.1186/s13073-025-01496-8\#Sec37 \\
    MME         & https://github.com/ga4gh/mme-apis/tree/master/testing \\
    VPI               & https://www.nature.com/articles/ejhg2017123\#Sec9 \\
    ADX                    & https://link.springer.com/article/10.1186/s13023-019-1040-6\#Sec37 \\
    RAMEDIS              & http://www.ramedis.de \\
    PUMCH          & https://zenodo.org/records/10774650 \\
    ZJUMCH (in-house)                               & -- \\
    \bottomrule
\end{tabularx}
